# Supplementary material for: ImOV3D: Learning Open-Vocabulary Point Clouds 3D Object Detection from Only 2D Images
Source: arXiv:2410.24001 source file (2024-10-31)
Supplement: Supplementary file 1 [file 10_supp.tex]

\newpage

\begin{center}
\Large \textbf{Supplementary Materials}
\end{center}

\section*{I. Supplementary Method Details}
This part supplements the methods mentioned in the main paper with detailed implementations and theoretical underpinnings.\newline

\textbf{Partial-View Removal:}
To obtain a point cloud from a 2D image, we first use a monocular depth estimation model ZoeDepth \cite{bhat2023zoedepth} to generate a depth map for the image, as shown in Fig \ref{fig:depth_color} (A). Inspired by \cite{zhang2023complete}, utilizing partial-view depth images for data augmentation serves to bolster the robustness and generalization capabilities of machine learning models in computer vision tasks. By simulating realistic occlusions and offering a diverse array of viewpoints, this approach prepares models to handle real-world variability and complexity more effectively, improving their performance across a wide range of scenarios.

In this process, we start by defining the point cloud and the camera viewpoints. The point cloud is a collection of points, which is formally represented as:
\begin{equation}
P = \{p_1, p_2, \ldots, p_n\}
\end{equation}
where each point $p_i$ is a part of the 3D object or scene we are interested in.

We consider two distinct viewpoints, A and B, characterized by their camera parameters $\theta_A$ and $\theta_B$, respectively. These parameters include the position and orientation of the camera that define each viewpoint.

Initially, we observe the point cloud from viewpoint A, resulting in a subset of points observed from this specific viewpoint, taking into account potential occlusions and the camera's field of view. This subset is denoted as:
\begin{equation}
P_A = \text{view}(P, \theta_A)
\end{equation}

Next, we change our perspective to viewpoint B and observe the point cloud again, which gives us another subset of points, denoted as:
\begin{equation}
P_B = \text{view}(P, \theta_B)
\end{equation}

The key step in this process involves identifying the overlapping points that are visible from both viewpoints A and B. This overlapping set is represented as:
\begin{equation}
P_{AB} = P_A \cap P_B
\end{equation}

After identifying the overlapping points, we proceed to remove these points from the subset observed from viewpoint A. The final set of points, after removing the overlapping ones, is represented as:
\begin{equation}
P_{A'} = P_A - P_{AB}
\end{equation}

Finally, this processed point cloud is rendered back into a depth image from viewpoint A. The resulting depth image, which includes holes where the overlapping points were removed, as shown in Fig \ref{fig:depth_part} (B), illustrating the effect of occlusions, is obtained through the rendering process, expressed as:
\begin{equation}
I_{A'} = \text{render}(P_{A'}, \theta_A)
\end{equation}

\begin{figure}[h]
    \centering
    \includegraphics[width=0.8\linewidth]{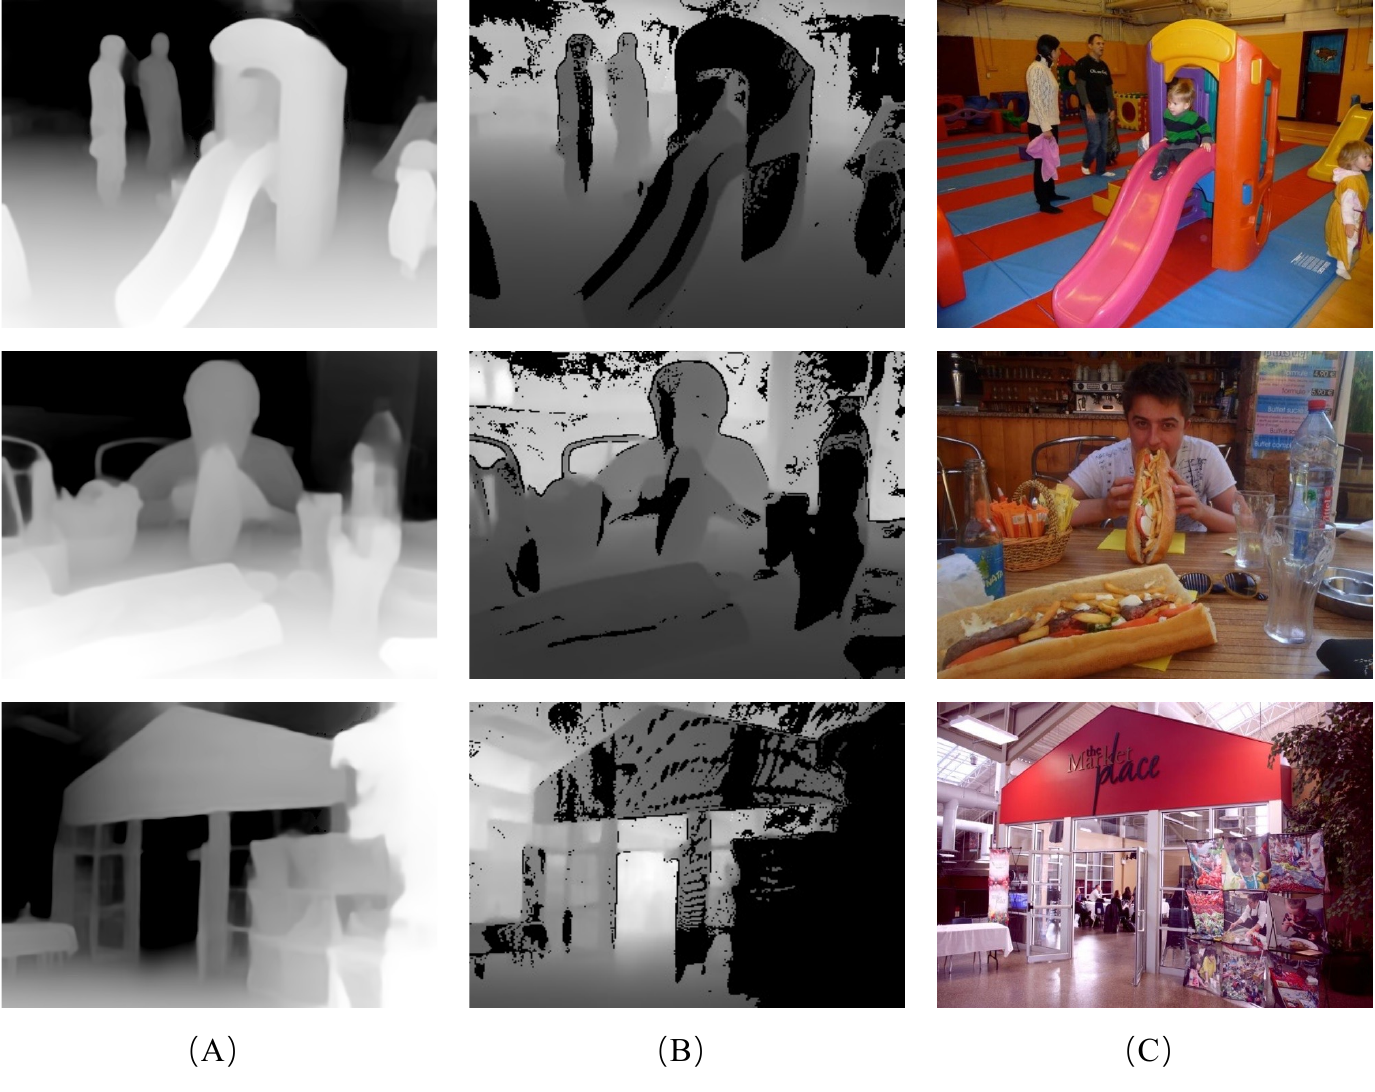}
    \caption{Illustration of (A) Depth Images, (B) Rendered Point Cloud Images after Partial-View Removal, and (C) Ground Truth 2D Images}
    \label{fig:depth_part}
\end{figure}

\textbf{Normal Estimator:}
In this paper, we employ Normal Estimator \cite{bae2021estimating} for surface normal estimation.

The process of normal estimation begins with the calculation of the surface normal vector at each pixel, a crucial step for understanding the orientation of surfaces in a scene. This calculation is conducted using a normal estimation model that utilizes either depth information or the 3D coordinates of each point in the scene. Mathematically, the surface normal vector at a point is defined as a 3D vector $\vec{N} = (N_x, N_y, N_z)$, where $\vec{N}$ represents the direction perpendicular to the surface at that pixel, as shown in the equation
\begin{equation}
\vec{N} = (N_x, N_y, N_z).
\end{equation}
Following the estimation of normal vectors across the scene, the next phase involves the extraction of horizontal normal vectors $\vec{N_i}$ at each pixel. This selection process focuses on vectors that align with the horizontal plane of the scene, essential for applications such as ground plane detection or horizon line estimation. Once horizontal normal vectors are identified, they undergo a clustering process to find a consensus on the predominant horizontal surface orientation within the scene. This process yields $\vec{N_{pred}}$, a vector representing the normal to the horizon surface, encapsulated by the equation
\begin{equation}
\vec{N_{pred}} = \text{Clustering}(\vec{N_i}).
\end{equation}
The final step in the normal estimation process is the alignment of $\vec{N_{pred}}$ with the Z-axis of the coordinate system to ensure a standardized representation of orientation. Achieving this alignment involves calculating a rotation matrix $R$, which, when applied to $\vec{N_{pred}}$, orients the vector parallel to the Z-axis. This is crucial for maintaining consistent orientation representation across different scenes and supports applications requiring a fixed reference frame. The alignment can be mathematically represented as
\begin{equation}
\vec{N_{aligned}} = R \cdot \vec{N_{pred}},
\end{equation}
where $\vec{N_{aligned}}$ is the resulting vector aligned with the Z-axis, ensuring a uniform approach to interpreting surface orientations in various applications.

\textbf{3D Box Filtering Module:}
Similar to \cite{zhang2023opensight}, this module's goal is to improve annotation quality by converting 2D bounding boxes into their 3D counterparts for objects within indoor scenes. This conversion process is pivotal for achieving a more accurate spatial representation of objects. However, the transition from 2D to 3D can introduce discrepancies between the generated 3D bounding boxes and the objects' actual dimensions. To mitigate this, we employ Large Language Models (LLMs), such as GPT-4 \cite{achiam2023gpt}, to obtain size priors for various object categories encountered in indoor environments. GPT-4\cite{achiam2023gpt}'s capability to provide reliable size estimates ensures that the adjusted 3D bounding boxes more closely align with the real-world sizes of objects, thereby enhancing the precision of annotations in indoor scene analysis.

\clearpage
\section*{II. Unexpanded Category AP Analysis}
This section provides a detailed discussion on the 20 categories within the SUNRGBD\cite{sunrgbd} and ScanNet \cite{scannet} datasets that were not fully explored in the main paper. 

Table \ref{tab:20scan} and Table \ref{tab:20sun} corresponds to Table \ref{tab:main_table1} in the main paper.

Table \ref{tab:adapscan} and Table \ref{tab:adapsun} corresponds to Table \ref{tab:main_table2} in the main paper.

\begin{table}[h]
    \centering
    
    \resizebox{1\linewidth}{!}{
    \begin{tabular}{l|c|cccccccccc}
    \toprule
Methods& \textbf{Mean} & toilet              & bed                 & chair               & sofa                & dresser            & table               & cabinet            & bookshelf          & pillow              & sink               \\
\midrule
OV-VoteNet~\cite{VoteNet} & 5.86 & 17.36                        & 25.83                        & 0.54                        & 28.85                         & 0.02                        & 0.94                        & 0.19                        & 0.0027                        & 2.75                           & 5.32                                                                      \\
OV-3DET~\cite{ov3det} & 5.69 & 23.44 & 22.39 &  7.07 &  24.15 &  0.98 & 0.21 &  0.12 &  0.03 &  0.18 &  1.35     \\
  
OV-3DETR~\cite{3DETR} & 5.3 & 25.34                        & 10.12                        & 1.11                        & 28.2                         & 0.001                        & 0.05                        & 0.029                        & 0.0001                        & 3.05                           & 2.34                                                                      \\
\textbf{ImOV3D} (Ours) & \textbf{12.64} & 55.86 & 28.82 &  11.72 &  28.16 &  0.453 & 7.44 &  1.23 &  0.05 &  4.42 &  29.12     \\

  \midrule
 Methods & & bathtub             & refrigerator       & desk                & nightstand          & counter            & door               &  curtain & box                & lamp               & bag                               \\
OV-VoteNet~\cite{VoteNet} &  & 18.71                        & 7.63                        & 2.2                        & 0.0059                         & 0.04                        & 0.29                        & 1.16                        & 0.02                        & 5.28                           & 0.03                                                                      \\
OV-3DET~\cite{ov3det} &  & 16.98 & 3.1 &  0.1 &  0.0012 &  0.12 & 0.12 &  4.15 &  7.2 &  2.1 &  0.1     \\
  
OV-3DETR~\cite{3DETR} &  & 24.68                        & 4.24                        & 1.6                        & 0.0034                         & 0.02                        & 0.47                        & 1.45                        & 0.016                        & 2.23                           & 1.01                                                                      \\
\textbf{ImOV3D} (Ours) & & 43.61 & 14.90 &  13.05 &  0.09 &  0.17 & 1.77 &  0.53 &  0.56 &  10.34 &  0.50     \\
    \bottomrule
    \end{tabular}
    }
    \caption{Comparison of Average Precision (AP) Scores for 20 Specific Categories on the ScanNet\cite{scannet} Dataset During the Pretraining Stage. `Mean' represents the average value of all the 20 categories.}
    \label{tab:20scan}
\end{table}

\begin{table}[h]
    \centering
    
    \resizebox{1\linewidth}{!}{
    \begin{tabular}{l|c|cccccccccc}
    \toprule
Methods& \textbf{Mean} & toilet              & bed                 & chair               & bathtub                & sofa            & dresser               & scanner            & fridge          & lamp              & desk               \\
\midrule
OV-VoteNet~\cite{VoteNet} & 5.18 & 25.16                        & 20.63                        & 1.59                        & 14.43                         &24.98                        & 0.0021                        & 0.001                        & 0.19                        &   1.69                         & 0.52                                                                      \\
OV-3DET~\cite{ov3det} & 5.47 & 21.92 & 16.94 &  11.18 &  12.74 &  16.81 & 1.674 &  0.89 &  4.12 &  5.60 &  0.88     \\
  
OV-3DETR~\cite{3DETR} & 5.24 & 33.50                        & 8.47                       & 2.61                        & 26.54                         & 17.05                       & 0.0003                        & 0.0001                        & 2.29                       & 0.73                           & 0.05                                                                     \\
\textbf{ImOV3D} (Ours) & \textbf{12.61} & 53.45 & 21.61 &  13.65 &  49.00 &  25.20 & 0.14 &  0.02 &  4.81 &  8.49 &  3.23     \\

  \midrule
 Methods & & table             & stand      & cabinet                & counter          & bin            & bookshelf               &  pillow & microwave                & sink               & stool                               \\
OV-VoteNet~\cite{VoteNet} &  & 0.5                        & 0.0004                        & 0.0057                        & 0.0007                         & 0.0007                        & 0.0008                        & 8.66                        & 0.01                        & 5.1                           & 0.11                                                                     \\
OV-3DET~\cite{ov3det} &  & 1.08 & 0.12 &  0.89 &  0.93 &  0.0003 & 1.47 &  7.43 &  3.54 &  0.13 &  1.01     \\
  
OV-3DETR~\cite{3DETR} &  & 0.05                        & 0.0001                       & 0.0004                       & 0.0001                        & 0.0001                       & 0.0002                        & 9.51                        & 0.0001                        & 2.47                           & 1.63                                                                      \\
\textbf{ImOV3D} (Ours) & & 6.17 & 0.0011 &  0.0354 &  0.0022 &  12.22 & 0.0048 &  14.20 &  11.98 &  20.63 &  7.39     \\
    \bottomrule
    \end{tabular}
    }
    \caption{Comparison of Average Precision (AP) Scores for 20 Specific Categories on the SUNRGBD\cite{sunrgbd} Dataset During the Pretraining Stage. `Mean' represents the average value of all the 20 categories.}
    \label{tab:20sun}
\end{table}

\begin{table}[H]
    \centering
    
    \resizebox{1\linewidth}{!}{
    \begin{tabular}{l|c|cccccccccc}
    \toprule
Methods& \textbf{Mean} & toilet              & bed                 & chair               & sofa                & dresser            & table               & cabinet            & bookshelf          & pillow              & sink               \\
\midrule
OV-3DET~\cite{ov3det} & 18.02 & 57.29 & 42.26 &  27.06 &  31.5 &  8.21 & 14.17 &  2.98 &  5.56 &  23 &  31.6     \\
  
CoDA~\cite{coda} & 19.32 & 68.09                        & 44.04                        & 28.72                        & 44.57                         & 3.41                        & 20.23                        & 5.32                        & 0.03                        & 27.95                           & 45.26                                                                      \\
\textbf{ImOV3D} (Ours) & \textbf{21.45} & 79.23 & 52.07 & 29.25 & 60.20  & 0.47 & 21.67 & 2.21 & 1.37 & 23.50 & 42.02     \\

  \midrule
 Methods & & bathtub             & refrigerator       & desk                & nightstand          & counter            & door               &  curtain & box                & lamp               & bag                               \\
OV-3DET~\cite{ov3det} &  & 56.28 & 10.99 &  19.72 &  0.77 &  0.31 & 9.59 &  10.53 &  3.78 &  2.11 &  2.71     \\
  
CoDA~\cite{coda} &  & 50.51                        & 6.55                        & 12.42                        & 15.15                         & 0.68                        & 7.95                        & 0.01                        & 2.94                        & 0.51                           & 2.02                                                                      \\
\textbf{ImOV3D} (Ours) & & 51.39 & 25.65 & 30.11 & 0.39 & 0.66 & 1.05 & 0.07 & 2.94 & 2.70 & 2.13     \\
    \bottomrule
    \end{tabular}
    }
    \caption{Comparison of Average Precision (AP) Scores for 20 Specific Categories on the ScanNet\cite{scannet} Dataset During the Adaptation Stage. `Mean' represents the average value of all the 20 categories.}
    \label{tab:adapscan}
\end{table}

\begin{table}[h]
    \centering
    
    \resizebox{1\linewidth}{!}{
    \begin{tabular}{l|c|cccccccccc}
    \toprule
Methods& \textbf{Mean} & toilet              & bed                 & chair               & bathtub                & sofa            & dresser               & scanner            & fridge          & lamp              & desk               \\
\midrule

OV-3DET~\cite{ov3det} & 20.46 & 72.64 & 66.13 &  34.8 &  44.74 &  42.10 & 11.52 &  0.29 &  12.57 &  14.64 &  11.21     \\
\textbf{ImOV3D} (Ours) & \textbf{22.53}& 76.70 & 65.36 & 32.21 & 55.77 & 50.01 & 0.20 & 2.94 & 13.77 & 26.20 & 11.54      \\

  \midrule
 Methods & & table             & stand      & cabinet                & counter          & bin            & bookshelf               &  pillow & microwave                & sink               & stool                               \\

OV-3DET~\cite{ov3det} &  & 23.31 & 2.75 &  3.4 &  0.75 &  23.52 & 9.83 &  10.27 &  1.98 &  18.57 &  4.1     \\
\textbf{ImOV3D} (Ours)& &16.68 & 0.08 & 0.47 & 0.03 & 29.21 & 0.10 & 15.71 & 20.74 & 30.21 & 2.81     \\
    \bottomrule
    \end{tabular}
    }
    \caption{Comparison of Average Precision (AP) Scores for 20 Specific Categories on the SUNRGBD\cite{sunrgbd} Dataset During the Pretraining Stage. `Mean' represents the average value of all the 20 categories.}
    \label{tab:adapsun}
\end{table}

\newpage
\section*{III. Evaluating the efficiency of GPT-4 in the 3D box filtering module}

In this section, we will discuss the efficiency of GPT-4 \cite{achiam2023gpt} in the 3D box filtering module. In order to have a good comparison, we choose the SUNRGBD \cite{sunrgbd} as a visualizing dataset. To clearly demonstrate the results, we select the top 10 classes with the most instances in the validation set as our visualization targets. 

The volume ratio for these 10 classes is defined as \( \text{Ratio}_V = \frac{L \times W \times H}{(L_{\text{GT/GPT}} \times W_{\text{GT/GPT}} \times H_{\text{GT/GPT}})} \). The volume ratio provides an insightful metric to compare the performance of the 3D box filter module powered by GPT-4 \cite{achiam2023gpt} with the ground truth (GT). A ratio close to 1 indicates that the volume of the predicted box is very similar to the true value, indicating high precision. By calculating the volume ratio \( \text{Ratio}_V \) for each instance, we gather statistical data and use Kernel Density Estimation (KDE) to analyze and plot the distributions of the volume ratios.  Results are presented in Figure \ref{fig:volume_statistics_comparison}.

\begin{figure}[h]
    \centering
    \includegraphics[width=1\linewidth]{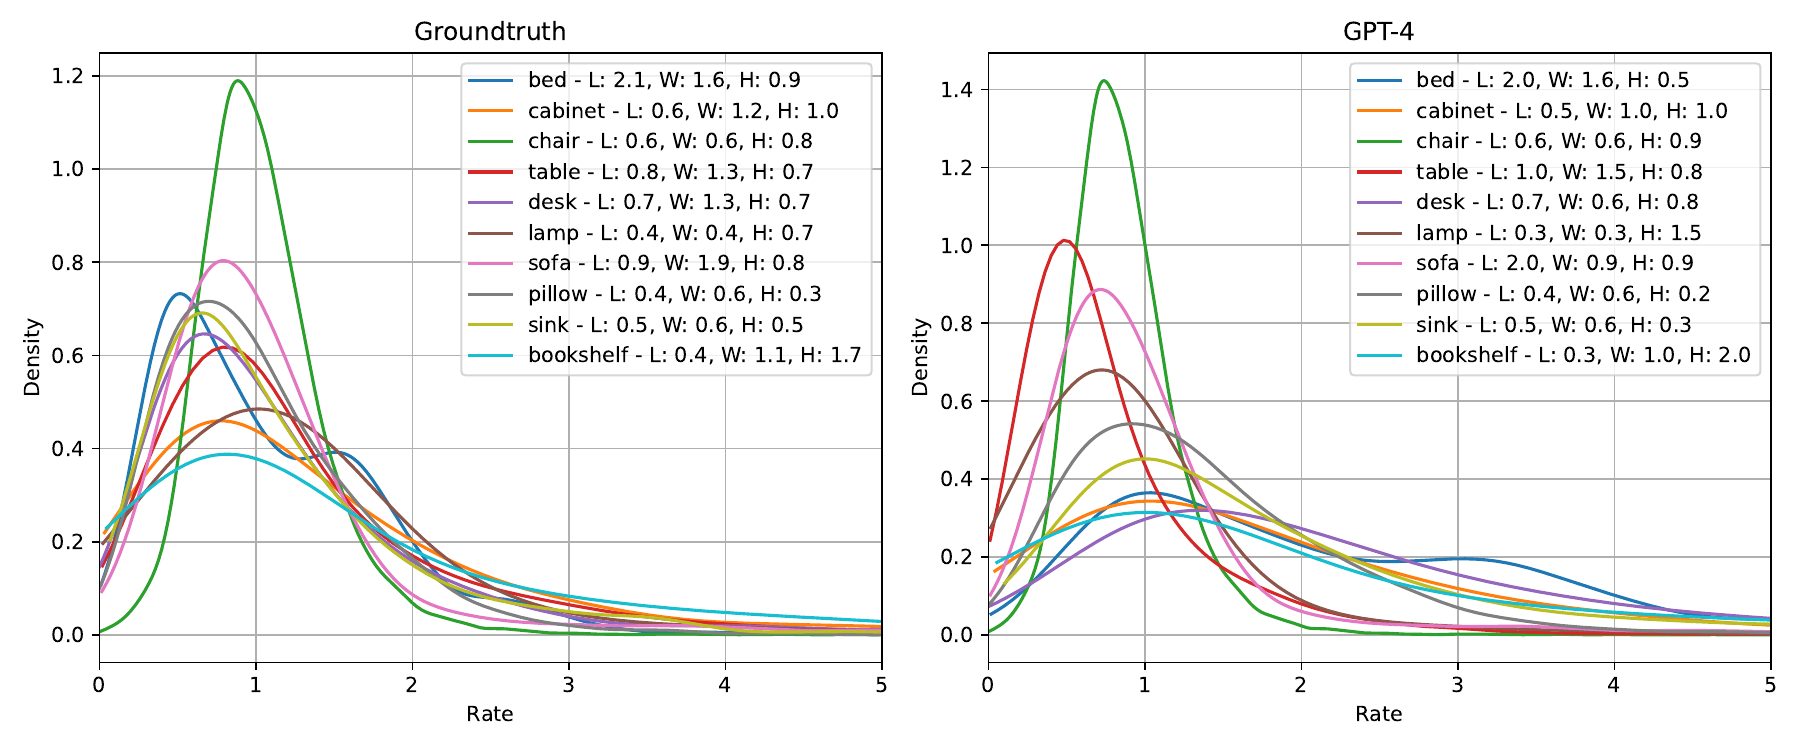}
    \caption{
Comparison of Volume Ratios: This image shows the efficiency of GPT-4 \cite{achiam2023gpt} using the SUNRGBD dataset by comparing volume ratios of the top 10 classes using Kernel Density Estimation (KDE).}
    \label{fig:volume_statistics_comparison}
\end{figure}

Figure \ref{fig:volume_statistics_comparison} fully demonstrates the effectiveness of the meansize database constructed by GPT-4 \cite{achiam2023gpt}. Subsequently, we used the constructed meansize in the 3D box filtering module to filter $\mathcal{B}_{3Dpseudo}$, with the results shown in Figure \ref{fig:visualof3Dboxfiler}.

\begin{figure}[h]
    \centering
    \includegraphics[width=1\linewidth]{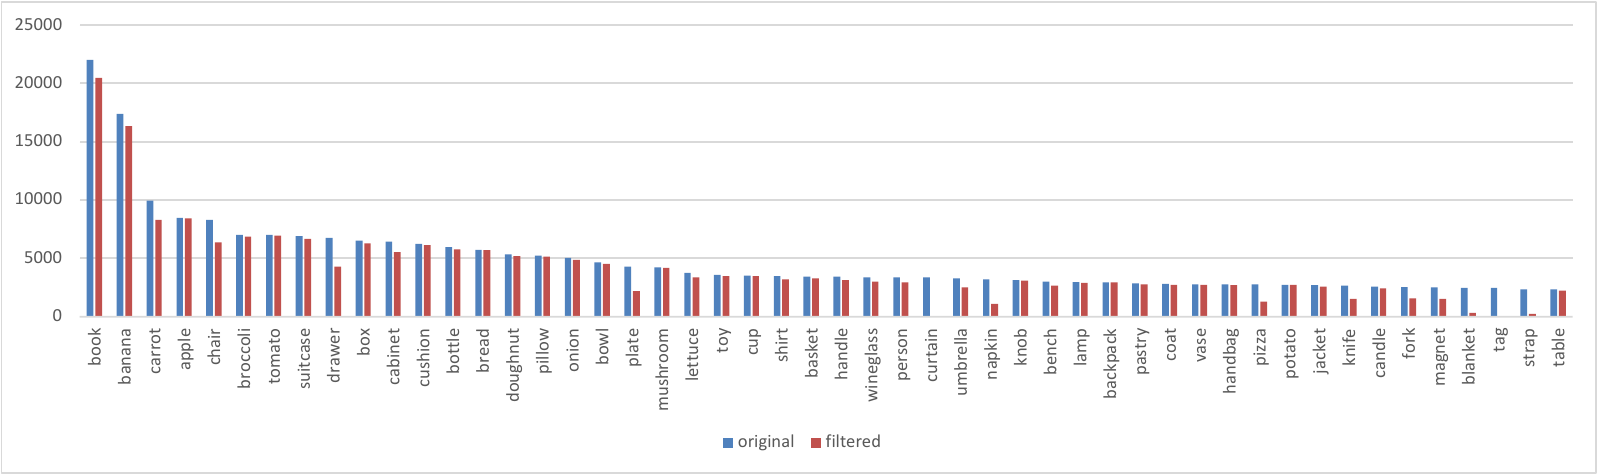}
    \caption{Results of Using the Meansize Database in the 3D Box Filtering Module: This figure shows the outcome of applying the meansize database constructed by GPT-4 \cite{achiam2023gpt} in the 3D box filtering module to filter $\mathcal{B}_{3Dpseudo}$ with a threshold $T=0.1$. The figure presents the number of 3D box of the top 50 classes with the most instances. The results highlight the efficiency and accuracy of the GPT-constructed meansize in improving the performance of the filtering process.}
    \label{fig:visualof3Dboxfiler}
\end{figure}

\newpage
\section*{IV. Detailed Experimental Implementation}
\subsection*{IV.A Fine-tuning Model Details (Detic \cite{detic} and ControlNet \cite{zhang2023adding})}
This subsection delves into the model adjustment and parameter selection process during the fine-tuning phase.\newline

\textbf{Detic \cite{detic}:} To finetune Detic \cite{detic} for our specific application, we first need to clarify the necessity for such an adjustment. The off-the-shelf Detic model is designed and optimized for ground truth images. However, our requirement for Detic \cite{detic} significantly diverges because it is to be utilized within the 2D OV Detector component of our ImOV3D project. In this component, the images we use are not ground truth images but pseudo images generated through ControlNet \cite{zhang2023adding}. Such images differ visually from ground truth images, which could potentially affect the detection performance of the Detic\cite{detic} model.

Given this, we decided to finetune Detic \cite{detic} to better suit our specific scenario. The finetuning process involves replacing the annotations based on ground truth images, which the Detic \cite{detic} model originally uses, with annotations from a 2D dataset that are accurate for our ControlNet-generated pseudo images. This replacement is aimed at enabling Detic \cite{detic} to more accurately recognize and process objects within these generated images, considering they differ in quality and characteristics from the real images used in the model's initial training.

Several key steps are involved in this finetuning process. First, we need to collect and prepare annotated data from the 2D dataset that applies to our pseudo images. Then, we use these annotations in the training process of the Detic \cite{detic} model to adapt it to our unique image characteristics. Through this process, we ensure that the Detic \cite{detic} model maintains efficiency and accuracy when dealing with images generated through ControlNet \cite{zhang2023adding}, thereby maximizing its efficacy in our ImOV3D project.

Finetuning the Detic \cite{detic} model not only improves its performance on specific images but also further validates the feasibility and flexibility of our approach. This process illustrates that by meticulously adjusting and optimizing model parameters in the face of varying application scenarios, we can effectively enhance the model's performance and adaptability. \newline

\textbf{ControlNet \cite{zhang2023adding}:} 
The objective of finetuning ControlNet \cite{zhang2023adding} is to add color to the rendered point cloud images. Originally, point cloud data lacks color information, meaning the depth images projected from these point clouds are also devoid of color. However, in many applications including but not limited to 3D reconstruction, augmented reality (AR), and virtual reality (VR), rich color and texture information are crucial for enhancing the visual quality of the final images. This necessitates the finetuning of ControlNet \cite{zhang2023adding}.

The finetuning process requires two types of data: original images and target images. In our scenario, the original images are depth images obtained by rendering point cloud after partial-view removal, as shown in Fig \ref{fig:depth_part} (B). While these depth images accurately represent the geometric information of the scenes, they lack color information. The target images, on the other hand, are ground truth 2D images corresponding to the point cloud data, as shown in Fig \ref{fig:depth_part} (C), containing the rich color and texture information we aim to incorporate.

During the finetuning of ControlNet \cite{zhang2023adding}, we do not use any text prompts but instead adhere to the official parameter settings recommended by ControlNet \cite{zhang2023adding}. We train the model for 180 epochs, through which the model learns how to effectively map the color information from the target images onto the corresponding depth images. This process not only enhances the visual appearance of the rendered images, making them more realistic and rich, but also improves the model's capability to handle color and texture variations across different scenes.

Through such finetuning, ControlNet \cite{zhang2023adding} can more accurately colorize depth images rendered from point clouds, preserving the geometric details from the original point cloud data while also integrating real-world color and texture characteristics. Such improvements are extremely beneficial for subsequent 3D vision applications, such as scene understanding and interaction in 3D. In summary, the process of finetuning ControlNet \cite{zhang2023adding} is a meticulous attempt to adjust and optimize model performance, aiming to achieve better results in handling specific tasks.

% \newpage

\newpage
\subsection*{IV.B Main Experiment and Baseline Experiment Details}
It outlines the setup and execution process of the main experiment, including comparisons with baseline experiments.

We detail and present four sets of key pretraining parameters. Table \ref{tab:training-params} showcases the training configuration for the ImOV3D method, an improved model we propose. Table \ref{tab:ov-votenet} provides a detailed description of the training parameters for OV-VoteNet\cite{VoteNet}, serving as another baseline model. Table \ref{tab:3detr} focuses on OV-3DETR \cite{3DETR}, presenting its specific training settings. Finally, Table \ref{tab:training-config-params-two-phases} outlines the training parameter details for the OV-3DET \cite{ov3det} model. These four tables aim to clearly display the specific parameter settings of each method during the pretraining stage, offering a direct perspective for comparison to the readers.

Table \ref{tab:adaptation-params} presents the parameter configurations of our experiments during the adaptation stage.
\begin{table}[h]
\centering
\caption{Key Parameters for ImOV3D Pretraining Configuration}
\label{tab:training-params}
\begin{tabular}{l l l}
\toprule
\textbf{Parameter} & \textbf{Value} & \textbf{Description} \\
\midrule
\texttt{--tower\_weights} & 0.3, 0.3, 0.4 & Fusion weights for different input modalities \\
\texttt{--batch\_size} & 12 & Number of samples per batch \\
\texttt{--learning\_rate} & 0.001 & Initial rate for model training \\
\texttt{--weight\_decay} & 0 & L2 regularization coefficient \\
\texttt{--max\_epoch} & 180 & Total number of pretraining training epochs \\
\texttt{--lr\_decay\_steps} & 80, 120, 160 & Epochs where learning rate decays \\
\texttt{--lr\_decay\_rates} & 0.1, 0.1, 0.1 & Learning rate decay factors \\
\bottomrule
\end{tabular}
\end{table}

\begin{table}[h]
\centering
\caption{Key Parameters for OV-VoteNet Pretraining Configuration}
\label{tab:ov-votenet}
\begin{tabular}{l l l}
\toprule
\textbf{Parameter} & \textbf{Value} & \textbf{Description} \\
\midrule
\texttt{--pc\_only\_weight} & 1 & Point clouds only input \\
\texttt{--batch\_size} & 12 & Number of samples per batch \\
\texttt{--learning\_rate} & 0.001 & Initial rate for model training \\
\texttt{--weight\_decay} & 0 & L2 regularization coefficient \\
\texttt{--max\_epoch} & 180 & Total number of pretraining training epochs \\
\texttt{--lr\_decay\_steps} & 80, 120, 160 & Epochs where learning rate decays \\
\texttt{--lr\_decay\_rates} & 0.1, 0.1, 0.1 & Learning rate decay factors \\
\bottomrule
\end{tabular}
\end{table}

\begin{table}[h]
\centering
\caption{Key Parameters for OV-3DETR Pretraining Configuration}
\label{tab:3detr}
\begin{tabular}{l l p{5cm}}
\toprule
\textbf{Parameter} & \textbf{Value} & \textbf{Description} \\
\midrule
\texttt{--max\_epoch} & 180 & Training duration in epochs. \\
\texttt{--base\_lr} & 7e-4 & Initial learning rate. \\
\texttt{--batchsize\_per\_gpu} & 12 & Samples per GPU. \\
\texttt{--weight\_decay} & 0.1 & L2 regularization. \\
\texttt{--warm\_lr} & 1e-6 & Warm-up learning rate. \\
\texttt{--warm\_lr\_epochs} & 9 & Duration of warm-up phase. \\
\texttt{--final\_lr} & 1e-6 & Learning rate for final phase. \\
\bottomrule
\end{tabular}
\end{table}

\begin{table}[h]
\centering
\caption{Key Parameters for OV-3DET Pretraining Configuration}
\label{tab:training-config-params-two-phases}
\begin{tabular}{l c c}
\toprule
\textbf{Parameter} & \textbf{Local Phase} & \textbf{DTCC Phase} \\
\midrule
\texttt{--max\_epoch} & 200 & 50 \\
\texttt{--nqueries} & 128 & 128 \\
\texttt{--base\_lr} & 4e-4 & 1e-4 \\
\texttt{--warm\_lr\_epochs} & - & 1 \\
\texttt{--batchsize\_per\_gpu} & 12 & 12 \\
\texttt{--final\_lr} & 1e-5& 1e-5 \\
\bottomrule
\end{tabular}
\end{table}

\begin{table}[h]
\centering
\caption{Key Parameters for ImOV3D Adaptation Configuration}
\label{tab:adaptation-params}
\begin{tabular}{l l l}
\toprule
\textbf{Parameter} & \textbf{Value} & \textbf{Description} \\
\midrule
\texttt{--tower\_weights} & 0.3, 0.3, 0.4 & Fusion weights for different input modalities \\
\texttt{--batch\_size} & 12 & Number of samples per batch \\
\texttt{--learning\_rate} & 0.0005 & Initial rate for model training \\
\texttt{--weight\_decay} & 0 & L2 regularization coefficient \\
\texttt{--max\_epoch} & 100 & Total number of adaptation training epochs \\
\texttt{--lr\_decay\_steps} & 40, 80 & Epochs where learning rate decays \\
\texttt{--lr\_decay\_rates} & 0.1, 0.1 & Learning rate decay factors \\
\bottomrule
\end{tabular}
\end{table}

\clearpage
\section*{V. Visualization Comparison during Pretraining Stage}

The visualization colors have specific meanings, and we're providing ImOV3D the prompt: "\textit{Please help me locate the \{category\}}". In the image, a bed is represented by red lines, a lamp by light green, a chair by pink, a table by blue, a sofa by purple, a pillow by orange, and a cabinet by dark green.

\begin{figure}[h]
    \centering
    \includegraphics[width=1\linewidth]{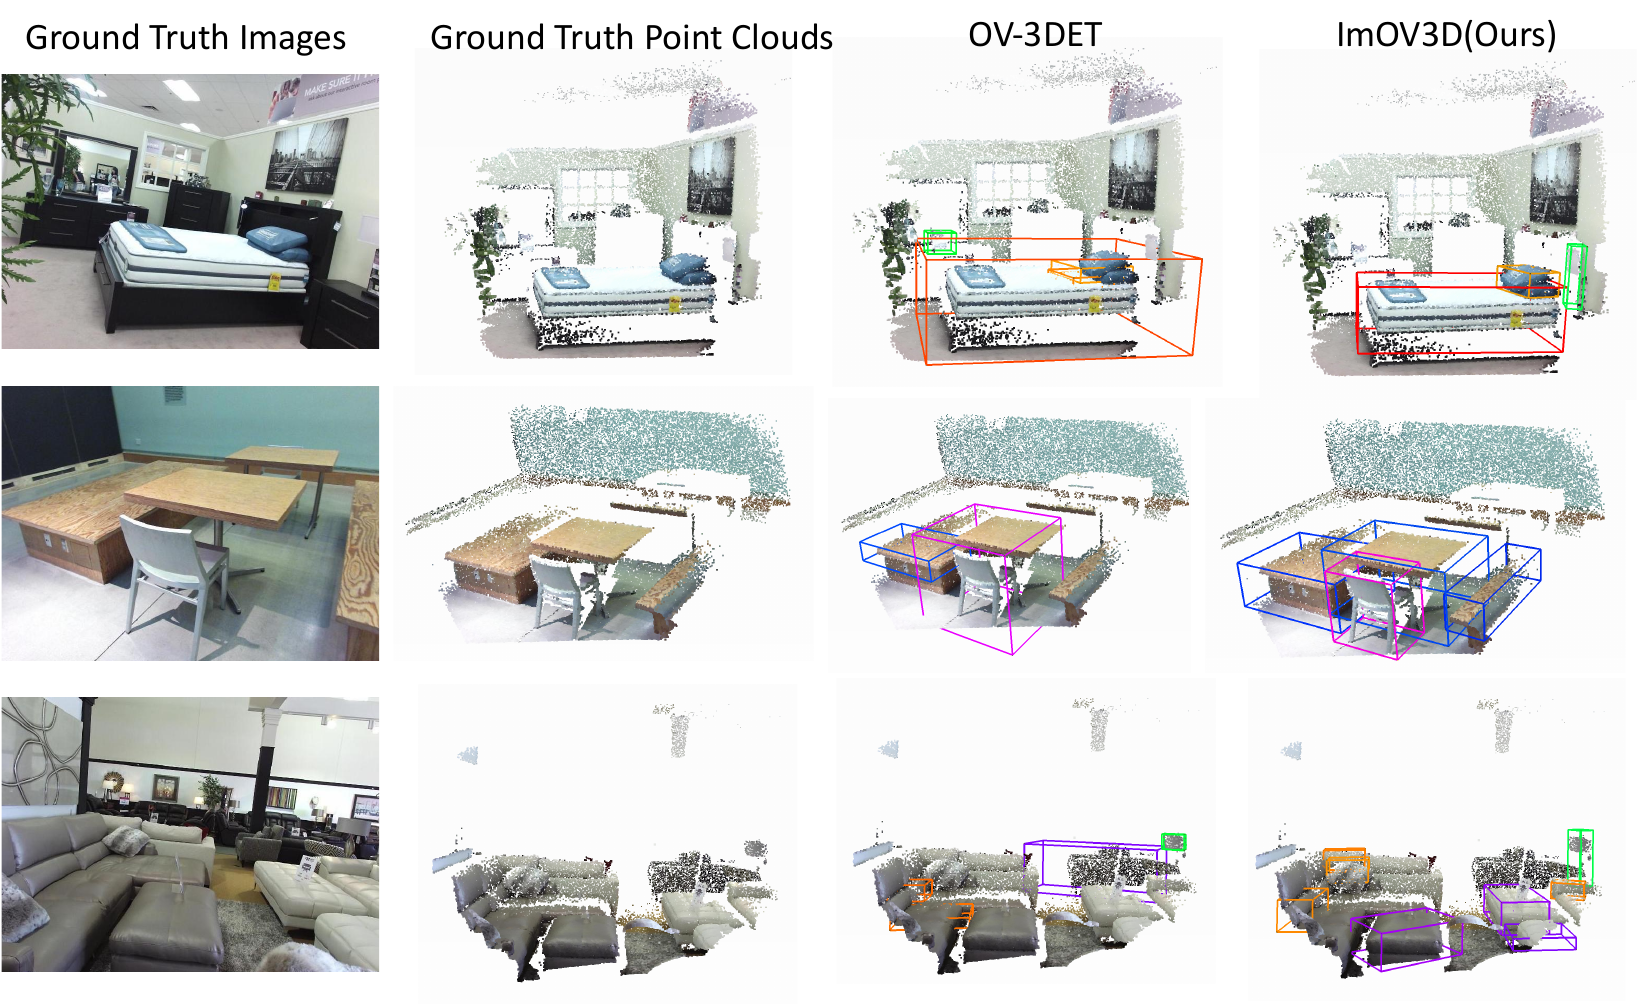}
    \caption{
During the pretraining stage, the visual comparison tested on the SUNRGBD\cite{sunrgbd} dataset includes four columns: the first column shows the ground truth images, the second column displays the ground truth point clouds, the third column presents the detection results by OV-3DET \cite{ov3det}, and the fourth column reveals the detection outcomes by ImOV3D.}
    \label{fig:sun_vis}
\end{figure}

\clearpage
\begin{figure}[t]
    \centering
    \includegraphics[width=1\linewidth]{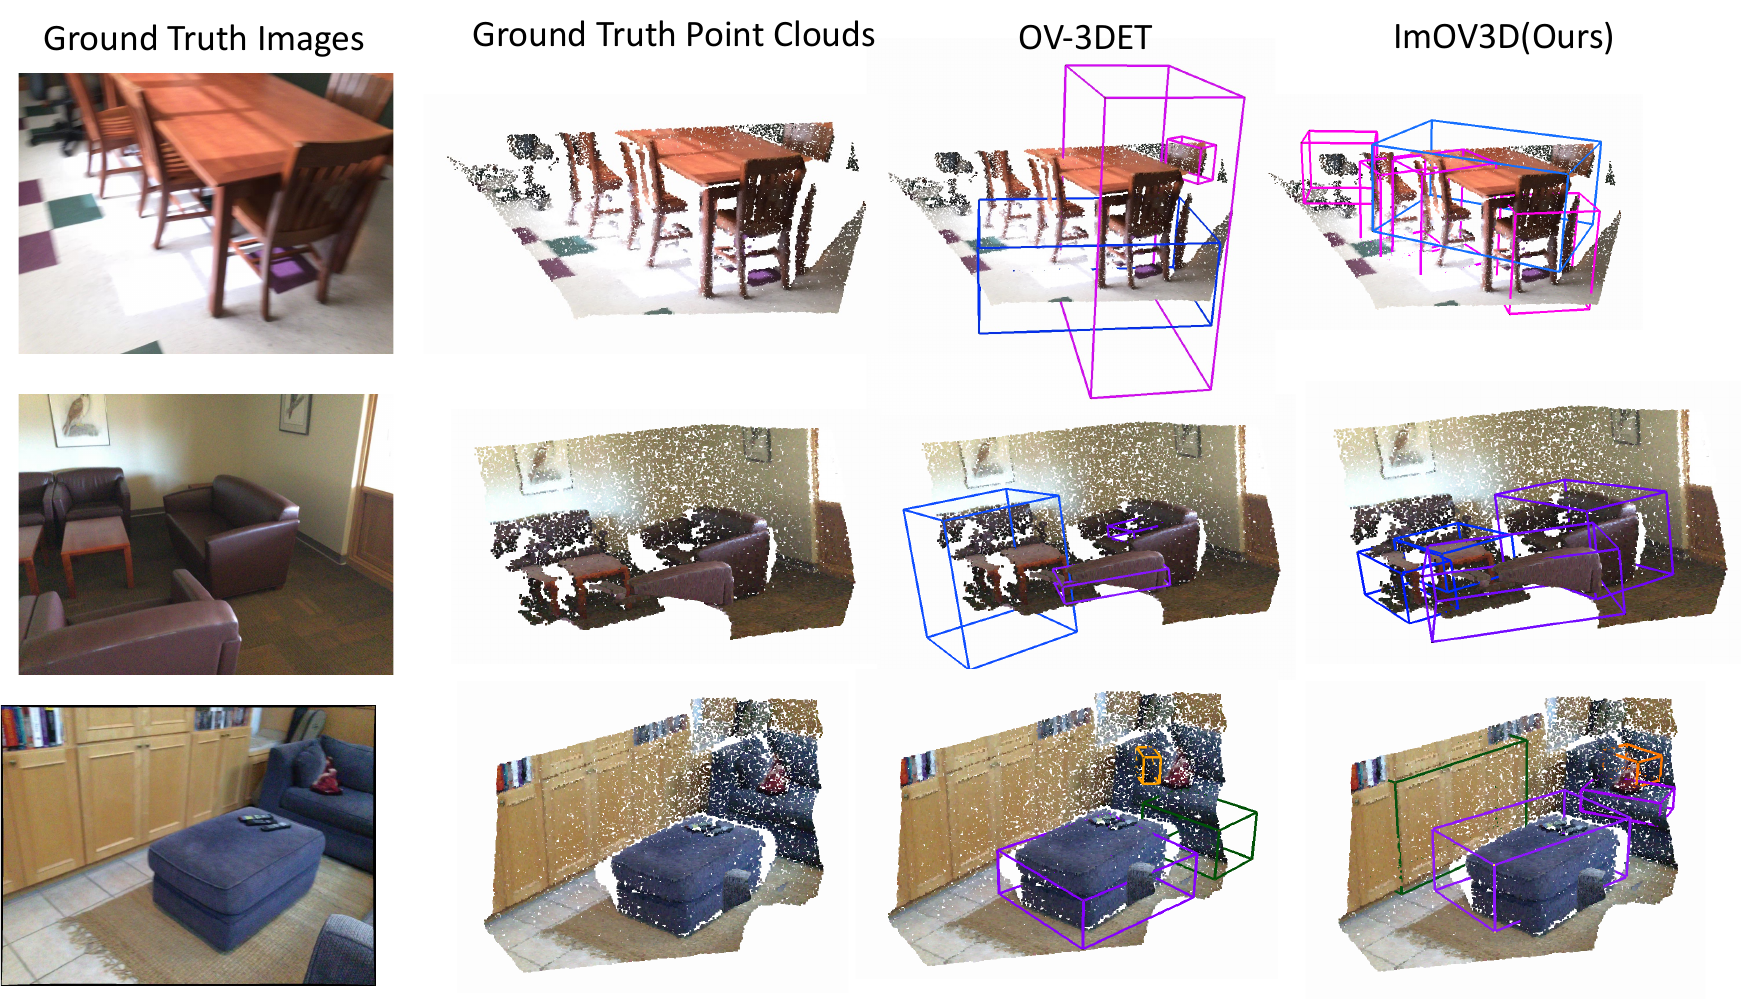}
    \caption{
During the pretraining stage, the visual comparison tested on the ScanNet \cite{scannet} dataset includes four columns: the first column shows the ground truth images, the second column displays the ground truth point clouds, the third column presents the detection results by OV-3DET\cite{ov3det}, and the fourth column reveals the detection outcomes by ImOV3D .}
    \label{fig:scan_vis}
\end{figure}

\clearpage
\section*{VI. Explanation of the formula for the Rotation Correction Module}

In this section, we explore Equation \ref{eq:HSANE1} in depth, utilizing Rodrigues' rotation formula. It calculates the rotation matrix \( R \in SO(3) \) for a rotation by \( \theta \) (less than \(180^\circ\)) around the axis defined by the unit vector \( \hat{n} = (n_x, n_y, n_z) \). The Rodrigues' rotation formula matrix is defined as:

\[
R = I + (\sin \theta) N + (1 - \cos \theta) N^2
\]

Where \( I \) is the identity matrix, and the skew-symmetric matrix \( N \) for the unit vector \(\hat{n}\) is constructed as:

\[
N = \begin{bmatrix}
0 & -n_z & n_y \\
n_z & 0 & -n_x \\
-n_y & n_x & 0
\end{bmatrix}
\]

To align unit vector \( N_{\text{pred}} \) with unit vector \( Z_{\text{pred}} \), we start from the definitions of the inner product and cross product:

\[
v = N_{\text{pred}} \times Z_{\text{pred}}
\]
\[
N_{\text{pred}} \cdot Z_{\text{pred}} = \cos\theta, \quad |N_{\text{pred}} \times Z_{\text{pred}}| = \sin\theta
\]

Thus, we have:

\[
v = N_{\text{pred}} \times Z_{\text{pred}} \quad \Rightarrow \quad v = \sin\theta \, \hat{n}
\]

Accordingly, define:

\[
K \stackrel{\mathrm{def}}{=} (\sin \theta) N = \begin{bmatrix}
0 & -n_z & n_y \\
n_z & 0 & -n_x \\
-n_y & n_x & 0
\end{bmatrix} = \begin{bmatrix}
0 & -v_z & v_y \\
v_z & 0 & -v_x \\
-v_y & v_x & 0
\end{bmatrix}
\]

Based on Rodrigues’ rotation formula, we have:

\[
R = I + K + \frac{1 - \cos \theta}{\sin^2 \theta} K^2 
\]

\[
= I + K + K^2 \frac{1 - N_{\text{pred}} \cdot Z_{\text{pred}}}{\|v\|^2} 
\]
